# Supplementary material for: Differential Dynamic Microscopy of Bacterial Motility
Source: arXiv:1004.4764 ancillary file (2010-10-02)
Supplement: Supplementary file 1 [file Supplementary_materials.pdf]

# Differential Dynamic Microscopy of Bacterial Motility (Supplementary Materials)

L. G. Wilson, V. A. Martinez, J. Schwarz-Linek, J. Tailleur, P. N. Pusey, and W. C. K. Poon
*SUPA and COSMIC, School of Physics & Astronomy,*
*The University of Edinburgh, Mayfield Road, Edinburgh EH9 3JZ, United Kingdom*

G. Bryant
*Applied Physics, School of Applied Sciences, RMIT University, Melbourne, Victoria 3000, Australia*
(Dated: October 1, 2010)

### Details of bacterial growth

The cells were *grown* at 30°C and **shaken** at 200 rpm in L-broth (tryptone 10.0 g/l, yeast extract 5.0 g/l, NaCl 5.0 g/l) for 16 h and re-inoculated 1:100 into T-broth (tryptone 10.0 g/l, NaCl 5.0 g/l). After 4 h cells were harvested in mid-exponential phase.

The motility buffer consisted of 6.2 mM $K_2HPO_4$, 3.8 mM $KH_2PO_4$, 67 mM NaCl, 0.1 mM EDTA, at pH=7.0.

### Extra plots of experimental and simulation data

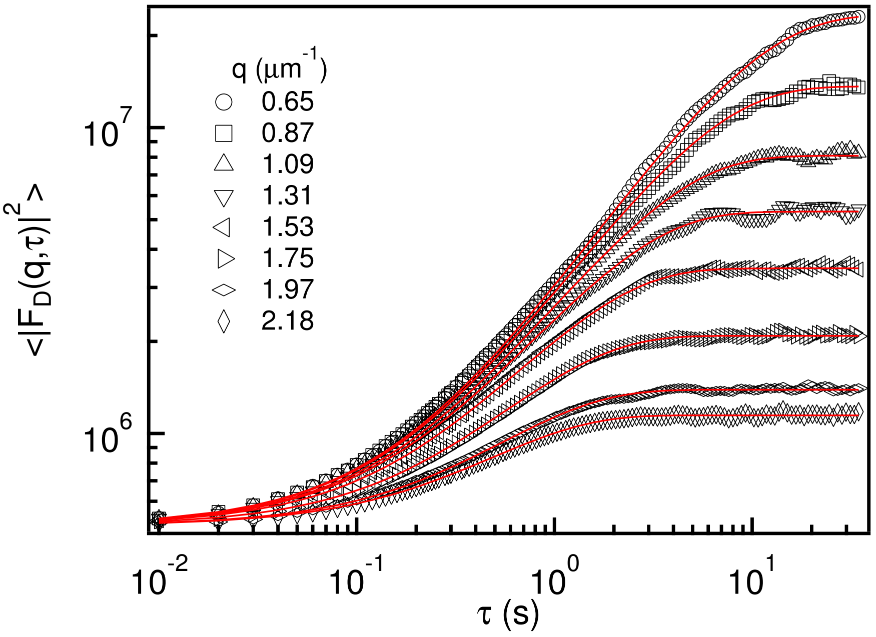


FIG. S.1: Measured DICFs (symbols) versus delay time for non-motile *motA* mutants of *E. coli* AB1157 for several values of $q$ spanning the whole available range (see key). Lines are fits using Eq. (7) with $f(q,\tau) = e^{-Dq^2\tau}$.

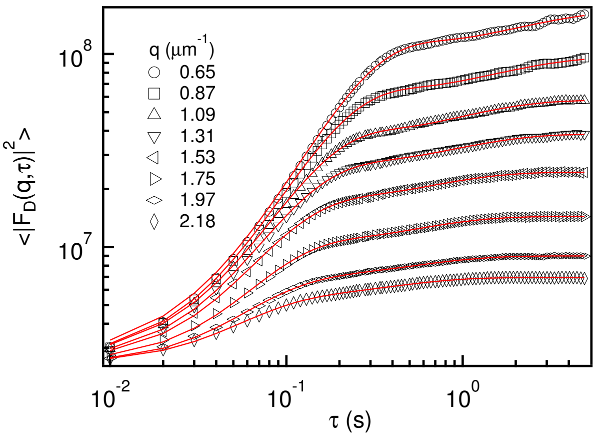


FIG. S.2: Measured DICFs (symbols) versus delay time for motile wild-type AB1157 *E.coli* for several values of $q$ spanning the whole available range (see key). Lines are fits using Eqs (7)-(11).

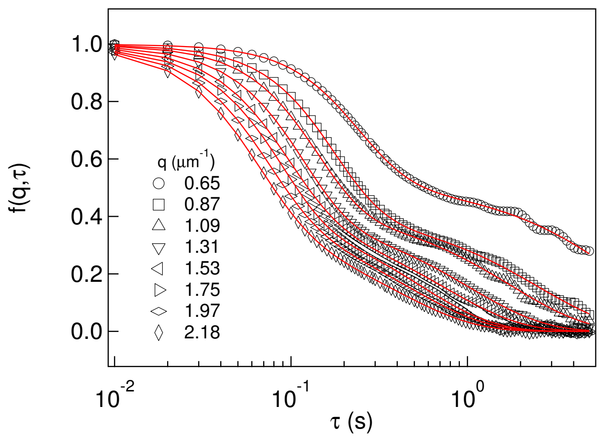


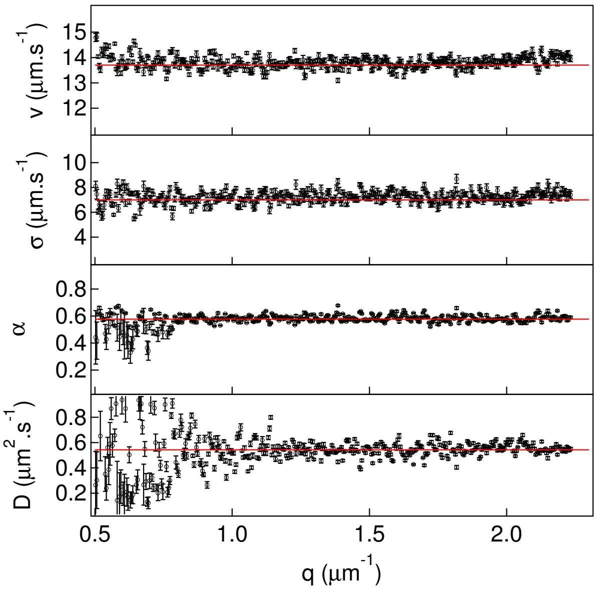


FIG. S.3: (Left, a) Reconstructed ISFs (symbols) and calculated ISFs (lines) obtained from fitting the DICFs calculated from simulated 'images' (see text) for several values of $q$ (see key). (Right, b) Parameters (symbols) extracted from fitting the DICFs as a function of $q$. From top to bottom: $v$ and $\sigma$ of the Schulz distribution, motile fraction $\alpha$ and diffusivity $D$. Lines are the input parameters used to create the time-lapsed simulated 'images': $\bar{v} = 13.7\mu\text{ms}^{-1}$ and $\sigma = 7\mu\text{ms}^{-1}$ in a Schulz distribution, $\alpha = 0.57$ and $D = 0.543\mu m^2/s$.
